# Supplementary material for: System Design for an Integrated Lifelong Reinforcement Learning Agent for Real-Time Strategy Games
Source: arXiv:2212.04603 source file (2022-12-08)
Supplement: Supplementary file 1 [file z.appendix.tex]

\section{Appendix}

\subsection{Starcraft 2 Task Variants}
\label{sec:sc2_task_descriptions}
The task variants we consider are as follows:

\begin{itemize}
    \item \textbf{Collect Mineral Shards – No Fog of War}: A map with 2 Marines and an endless supply of Mineral Shards. Rewards are earned by moving the Marines to collect the Mineral Shards, with optimal collection requiring both Marine units to be split up and moved independently. Whenever all 20 Mineral Shards have been collected, a new set of 20 Mineral Shards are spawned at random locations (at least 2 units away from all Marines). Fog of war is disabled. 
     \item \textbf{Collect Mineral Shards – Fog of war:} A map with 2 Marines and an endless supply of Mineral Shards. Rewards are earned by moving the Marines to collect the Mineral Shards, with optimal collection requiring both Marine units to be split up and moved independently. Whenever all 20 Mineral Shards have been collected, a new set of 20 Mineral Shards are spawned at random locations (at least 2 units away from all Marines). Fog of war is enabled, meaning the agent must be able to learn without full knowledge of the current state of the environment.
     \item \textbf{DefeatZerglingsAndBanelings – One Group:} A map with 9 Marines on the opposite side from a group of 6 Zerglings and 4 Banelings. Rewards are earned by using the Marines to defeat Zerglings and Banelings. Whenever all Zerglings and Banelings have been defeated, a new group of 6 Zerglings and 4 Banelings is spawned and the player is awarded 4 additional Marines at full health, with all other surviving Marines retaining their existing health (no restore). Whenever new units are spawned, all unit positions are reset to opposite sides of the map
     \item \textbf{DefeatZerglingsAndBanelings – Two Groups:} A map with 9 Marines in the center with two groups consisting of 9 Zerglings one one side and 6 Banelings on the other side. Rewards are earned by using the Marines to defeat Zerglings and Banelings. Whenever a group has been defeated, a new group of 9 Zerglings and 6 Banelings is spawned and the player is awarded 6 additional Marines at full health, with all other surviving Marines retaining their existing health (no restore). Whenever new units are spawned, all unit positions are reset to opposite sides of the map.
     \item \textbf{DefeatRoaches – One Group:} A map with 9 Marines and a group of 4 Roaches on opposite sides. Rewards are earned by using the Marines to defeat Roaches, with optimal combat strategy requiring the Marines to perform focus fire on the Roaches. Whenever all 4 Roaches have been defeated, a new group of 4 Roaches is spawned and the player is awarded 5 additional Marines at full health, with all other surviving Marines retaining their existing health (no restore). Whenever new units are spawned, all unit positions are reset to opposite sides of the map.
     \item \textbf{DefeatRoaches – Two Groups:} A map with 9 Marines in the center and two groups consisting of 6 total Roaches on opposite sides (3 on each side). Rewards are earned by using the Marines to defeat Roaches, with optimal combat strategy requiring the Marines to perform focus fire on the Roaches. Whenever all 6 Roaches have been defeated, a new group of 6 Roaches is spawned and the player is awarded 7 additional Marines at full health, with all other surviving Marines retaining their existing health (no restore). Whenever new units are spawned, all unit positions are reset to starting areas of the map.
\end{itemize}

\subsection{Implementation Details}
\label{exp:archs}

\subsubsection{Starcraft 2}
\label{sec:imp_sc2}

In this section we describe the implementation details for our \SC{} agent and experiments. The wake agent is a VTrace agent \citep{espeholt2018impala}. The feature extractor component of the wake agent consists of an architecture that is a slight modification of the FullyConv model of \citet{vinyals2017starcraft}. We further split this into a feature extractor component and a policy network component to facilitate easy weight copying between the wake and sleep agents. For the hidden replay model, we add a LayerNormalization layer to the output of the feature extractor to constrain the space of the features, which helps to improve feature reconstructions and limit feature drift. The architecture produces features of dimension 8192.

The sleep agent feature extractor and policy network architectures are identical to the wake model. We use a five-layer convolutional neural network architecture with for the encoder and a five-layer deconvolutional architecture for the decoder for the VAEs for the sequential and two-headed models. In both cases, we use ReLU activations between the layers and add batch normalization before the ReLUs. We use two-layered multi-layered perceptrons with ReLU activation functions for the encoder and decoder for the VAE for the hidden replay model. To improve numerical stability, the logvar predicted by the encoder is bounded to take values in $[-5, 5]$ using a scaled-hyperbolic tangent layer.

Three styles of replay are used during sleep for the hidden replay architecture: experience replay on a buffer of 10,000 observation-action pairs from a FIFO queue collected during the wake phase, generative replay on the feature vectors, and random replay. Only experience replay and generative replay is used to train the sleep agent for the sequential and two-headed architectures.

For the sequential architecture: the weight of the imitation loss (cross-entropy on action logits) is 50.0, the weight of the reconstruction loss is 1.0, and the weight of the KL loss of the VAE is 3.0. For the two-headed architecture: the weight of the imitation loss (cross-entropy on action logits) is 30.0, the weight of the reconstruction loss is 1.0, and the weight of the KL loss of the VAE is 2.0. For the hidden replay architecture: the weight of the imitation loss (cross-entropy on action logits) is 50.0, the weight of the reconstruction loss is 200.0, and the weight of the KL loss of the VAE is 5.0. These were determined via hand-tuning.

The agent enters sleep three times per task at even intervals for the sequential and two-headed architectures. The agent enters sleep twice per task at even intervals for the hidden replay architecture. Each training iteration of the wake model is trained on 32 trajectories. Each sleep consists of 4,500 iterations of training using batch sizes of 64 (64 wake samples, 64 generated samples, and 64 random observations from the random replay buffer). Generative replay is not used until the second sleep. 96 observations are selected randomly from the wake buffer every sleep to be added to the random replay buffer for the hidden replay architecture. When the agent wakes up, it resets the PPO model and offers advice with a 80\% probability linearly decaying to 0\% after for one-half the the duration between sleeps. No weight copying is used for the sequential variant, but weight copying (running a mini-evaluation block after sleep and copying the best Eigentask's parameters into the wake agent) and advice are both used for the two-headed and hidden replay variants.

The Adam optimizer is used to train both the wake and sleep agents with a learning rate of 1.0e-3. 

\textbf{Evaluation:} We selected 3 minigames involving battles  (\emph{DefeatRoaches} and \emph{DefeatZerglingsAndBanelings} tasks) or resource collection (\emph{CollectMineralShards}). We created two variants of each task, differentiated by the starting locations of units, the presence of ``fog-of-war'', and/or the number of friendly and enemy units. Task variants are described in Section~\ref{sec:sc2_task_descriptions}. We used PySC2 \citep{vinyals2017starcraft} to interface with SC-2. We used a subset of the available observation maps namely the unit type, selection status, and unit density two-dimensional observations. The action space is factored into functions and arguments, such as $\text{move}(x, y)$ or $\text{stop}()$. Following \citet{vinyals2017starcraft}, our policy networks output probabilities for the different action factors independently. %; outputs for arguments that do not apply to the chosen function are masked out. We prune the (very large) SC-2 action space down to a minimal set of functions necessary to complete all of the tasks.
%SC2 is especially challenging for lifelong RL because of its large action space, which requires selecting agents, specifying how to move agents via pointing and clicking, and enacting  task-specific actions such as firing weapons. 
The agent receives positive rewards for collecting resources and defeating enemy units, and negative rewards for losing friendly units. Single task experts (STEs) were trained to convergence ($\sim$ 30 million environment steps using the VTrace algorithm \citep{espeholt2018impala}). We consider the pairwise, alternating, and condensed scenarios where each LB consists of 2 million environment steps (about 6\% of the STE samples), and each EB consists of 30 episodes per task.

Each lifetime of a condensed scenario takes approximately 3-4 days running on systems with RTX2080 GPUs.

\subsection{Example Learning Curves for Lifelong Curricula on \SC{}}

\begin{figure}[H]
\centering
\includegraphics[width=0.95\textwidth]{figs/sc2_learning_curve_cropped.png}
\caption{Learning curve for our lifelong learning agent applied to a six minigame scenario in the \SC{} domain. Performance comparable to the converged single-task expert is \textasciitilde 100.}
\label{fig:sc2_learning_curves}
\end{figure}

\subsection{Understanding the Interplay Between Different Replay Mechanisms}
\label{sec:justification_of_exemplars}

We've observed that generative replay alone is not sufficient for the hidden replay architecture. This is because there is no constraint limiting the drift in the feature space between sleeps, so the feature extractor can completely change between two time steps if the tasks are perceptually dissimilar or dissimilar in policy. To help to overcome this issue, we employ ``random replay'' where we save a small batch of random observation-action pairs in the original observation space after every sleep, and randomly replay them during every sleep.  In Fig.\ \ref{fig:exemplar_replay_1}, we show the necessity of combining hidden replay with random replay. On the left, we see that using hidden replay without random replay results in the feature space for task 0 dramatically changing after training on task 1, and PM is low. On the right, we see that the distribution of task 0 before and after training on task 1 is significantly better aligned when hidden replay is used in conjunction with random replay, and PM significantly improves. Additional visualizations for pairs of dissimilar tasks are seen in Fig.~\ref{fig:exemplar_replay_2}. In Table \ref{tab:exemplars_vs_no_exemplars}, we see using random replay generally improves PM and FTR, which agrees with our hypothesis that it helps to maintain the feature space, leading to less forgetting and potentially features that generalize better to other tasks.

\begin{table}[H]
    \centering
    \begin{tabular}{|c|c|c|c|c|c|}
        \hline
         Scenario & Agent & PM & FT & BT & RP \\
         \hline
          Pairwise & No Random Replay & $-6.28$ ($ \pm 12.82$) & $1.35$ ($ \pm 0.24$) & $0.80$ ($ \pm 0.37$) & $1.08$ ($ \pm 0.19$) \\
         & Random Replay & $-3.03$ ($ \pm 4.92$) & $1.65$ ($ \pm 0.28$) & $0.92$ ($ \pm 0.13$) & $1.04$ ($ \pm 0.17$) \\
         \hline
        Condensed & No Random Replay & $-9.35$ ($ \pm 3.69$) & $1.37$ ($ \pm 0.15$) & $1.20$ ($ \pm 0.24$) & $1.16$ ($ \pm 0.16$) \\
         & Random Replay & $-3.05$ ($ \pm 1.76$) & $1.42$ ($ \pm 0.11$) & $1.00$ ($ \pm 0.03$) & $1.17$ ($ \pm 0.11$) \\
         \hline
    \end{tabular}
    \caption{Comparison of the hidden replay model with and without random replay. Results are averaged over multiple lifetimes, and we also record the standard deviation of the metrics.}
    \label{tab:exemplars_vs_no_exemplars}
\end{table}

\begin{figure}[H]
\centering
\includegraphics[width=0.8\textwidth]{figs/m18_exemplars.png}
\caption{We show the necessity of combining hidden replay with random replay. Left: Using hidden replay without random replay results in the feature space for task 0 dramatically changing after training on task 1, and the feature space for both classes converge to a point. PM is -10.68. Right: The distribution of task 0 before and after training on task 1 are significantly better aligned when hidden replay is used in conjunction with random replay. PM is -1.93.}
\label{fig:exemplar_replay_1}
\end{figure}

\begin{figure}[H]
\centering
\includegraphics[width=0.95\textwidth]{figs/m18_exemplars_2.png}
\caption{We show two examples where hidden + random replay maintains the feature space of the previous task after learning a new dissimilar SC-2 task (``Collect'' $\rightarrow$ ``Defeat'' and vice versa).}
\label{fig:exemplar_replay_2}
\end{figure}

\subsection{Applying STAM to SC-2}
\label{sec:stam_app}

In this section, we describe the details of how STAM can be applied for use in the SC-2 domain.

\paragraph{Background Removal (Preprocessing)}
As a preprocessing step, STAM includes a simple background removal method for SC-2 RGB observations based on erosion and dilation operations on images that exploits the simple structure of the background. The background largely stays the same under erosion and dilation operations, while objects become darker under erosion and brighter under dilation. So, we can extract objects and ignore patches with background by comparing eroded and dilated images and thresholding the background. The threshold is given by a hyperparameter "eps" which determines the threshold to eliminate noise (we suggest eps = 2 for SC-2). 

\paragraph{Feature Extraction}
With a given input (RGB Frames in this case) STAM begins by decomposing the image into a potential set of features in the form of overlapping patches. Instead of neurons or hidden layer units, STAM consists of STAM units – in its simplest form, a STAM unit functions as an online clustering module that operates directly on pixel space. Each STAM unit processes one patch, and the patches are overlapping, with a small stride to accomplish translation invariance (similar to CNNs). Patch size is based on the receptive field size, which is a hyperparameter. We used a single receptive field of $16\times16$ based on common object sizes that appear in tasks for SC-2. Therefore, we will assume a single receptive field size (STAM layer) for the rest of the report.

\paragraph{Centroid Learning (Learning)}
Every patch is clustered, in an online manner, to a set of centroids. Given the $m^{th}$ non-background input patch $x_m$ and set of centroids C, the nearest centroid $c_j$ is selected for patch $x_m$  as:
$$c_j=\text{argmin}_{(c \in C)} \; d(x_m, c)$$
Where $d(x_m,c)$ is the Euclidean distance between the patch $x_m$ and centroid c. The selected centroid is updated based on a learning rate parameter $\alpha$ as follows:
$$c_j = \alpha x_m + (1-\alpha) c_j, \;0<\alpha<1$$

\paragraph{Novelty Detection (Learning)}
When an input patch $x_m$ is significantly different than all centroids (i.e., its distance to the nearest centroid is a statistical outlier), a new centroid is created in C based on $x_m$. This function is necessary so that the architecture can learn novel features when the data distribution changes. To do so, we estimate in an online manner the distance distribution between input patches and their nearest centroid. The novelty detection threshold is defined as the 95th percentile ($\beta = 0.95$) of this distance distribution.

\paragraph{Dual-memory Organization (Learning)}
New centroids are stored temporarily in a Short-Term Memory (STM) of limited capacity $\Delta$. If an STM centroid $c_j$ is selected more than $\theta$ times, it is copied to the Long-Term Memory (LTM) for that layer. In the original STAM model, the LTM has (practically) unlimited capacity and a learning rate of zero. However, because of the much larger scale of the SC-2 data and tasks, LTM has been modified to have a fixed capacity. This memory organization is inspired by the Complementary Learning Systems framework where the STM role is played by the hippocampus and the LTM role by the cortex. %When STM is full, STAM replaces the least recently used centroid from the STM with the newly created centroid. When the LTM is full, a centroid from the  replaced with one of the most redundant existing centroids currently in the LTM. Here, redundancy simply means a centroid which is commonly chosen as a second choice match for another centroid. This memory organization is inspired by the Complementary Learning Systems framework where the STM role is played by the hippocampus and the LTM role by the cortex.  %When the LTM is full, a centroid is replaced with one of the most redundant existing centroids currently in the LTM.

\begin{figure}[h!]
    \centering
    \includegraphics[width=0.8\textwidth]{figs/embedding_rep.png}
    \caption{Summary of STAM output embedding creation}
    \label{fig:stam_embed}
\end{figure}

\paragraph{Embedding Creation (Post-processing)}
The centroids learned in the LTM often include shifted versions of the same qualitatively identifiable object due to the nature of extracting overlapping patches with a small stride Figure \ref{fig:stam_embed}-A. This means that each unique object has multiple centroids (with different ID’s) that are associated with it. In order to deal with this, we first pick the most central patch for each object to have an accurate localization Figure \ref{fig:stam_embed}-B. Second, we utilize centroid indices to assign object type identifiers for the central patches Figure \ref{fig:stam_embed}-C. We developed a voting-based method. Each central patch votes for k centroids that it would pick based on distance if its assigned centroid did not exist. Then using accumulated votes, STAM decides on object type identifiers for the centroids. This step is necessary because STAM can learn hundreds of centroids for a single type of object, and we need to map all of these centroids to a unique identifier for consistent representation. Once we assign object type identifiers, we have an output matrix-like Figure \ref{fig:stam_embed}-D.

\subsection{Validating Barlow Twins for SSRL using Object Detection}
\label{sec:barlow_app}
In this section, we provide evidence that Barlow Twins are well-suited as a self-supervised learning (SSL) algorithm for representation learning in the SC-2 domain. Table~\ref{tab:ssrl_od} shows the evaluation of the SSL trained backbones used in the Object Detection pipeline. To ensure that other components of the pipeline(RPN, ROI pooling) do not mask the contribution of the backbone, we ran the experiments on three pipelines (C4, FPN and DC5) offered by Detectron2\citep{wu2019detectron2}.
\begin{table}[H]
    \centering
    \begin{tabular}{|c|c|c|c|}
    \hline Backbone/Pipeline & C4 & FPN & DC5 \\
    \hline
         Barlow Twins & 12.943 & 42.641 & 6.083 \\
         MoCo & 6.083 & 43.110 & 6.675 \\
         Barlow Twins, initialized with ImageNet & 9.382 & 44.325 & 7.841 \\
         MoCo , initialized with ImageNet & 9.693 & 42.802 & 6.395 \\MoCo , initialized with ImageNet & 9.693 & 42.802 & 6.395 \\ 
         ImageNet & 14.903 & 42.107 & 6.885 \\
  \hline
    \end{tabular}
    \caption{Evaluation of SSL trained backbones using Object Detection as downstream task}
    \label{tab:ssrl_od}
\end{table}

        % \subsection{Single vs Multiple Eigentasks}
        % \label{sec:multieigen_app}
        % We explore the trade-offs in terms of lifelong learning metrics when using one versus multiple Eigentasks. We consider the case where the system encounters multiple tasks in sequence, and we evaluate the effect of the number of Eigentasks on the lifelong learning metrics. We trained the two-headed architecture for six lifetimes, each consisting of a random syllabi of three tasks with two million environment steps per task. We compared the effect of two Eigentasks vs one Eigentask and measured the \textit{differences} in terms of PM, FTR, BTR, and RP. We also measured standard deviation of the metrics. The results appear in Table \ref{tab:multi-eigentask}. We see that the multi-Eigentask system is higher in terms of FTR and BTR while negligibly lower in terms of PM and RP.

        % \begin{table}[H]
        %     \centering
        %     \resizebox{\textwidth}{!}{
        %     \begin{tabular}{|c|c|c|c|c|c|}
        %         \hline
        %           Setting & PM & FT & BT & RP \\
        %          \hline
        %          Two vs One Eigentask(s): Two-Headed Model & $-0.218$ ($ \pm 3.061$) & $0.197$ ($ \pm 0.092$) & $0.087$ ($ \pm 0.276$) & $-0.008$ ($ \pm 0.105$) \\
        %          \hline
        %     \end{tabular}
        %     }
        %     \caption{Differences between agents using the two-headed architecture with two Eigentasks vs one Eigentask averaged over six random condensed syllabi of three tasks.}
        %     \label{tab:multi-eigentask}
        % \end{table}

\subsection{Comparisons to Closest Model for Component Extensions}
\label{sec:closest_baseline}
In this section, we compare each component for extending the SC-2 system with its closest comparable model (i.e., a control model) to see how lifelong metrics are affected by adding the component. In all cases (excluding the condensed scenario for danger detection), we try to compare using the same set of syllabi between the baseline agent and extended agent with similar pre-training assumptions. Note that the Two-Headed Model is trained via wake-sleep phases whereas models based on ``Wake'' do not undergo sleep.

\subsubsection{Self-Monitoring Sleep w/ WATCH}

\begin{table}[H]
    \centering
    \resizebox{\textwidth}{!}{
    \begin{tabular}{|c|c|c|c|c|c|}
        \hline
         Scenario & Agent & PM & FT & BT & RP \\
         \hline
          Pairwise & Two-Headed Model & $-5.4$ ($ \pm 4.9$) & $1.13$ ($ \pm 0.25$) & $0.84$ ($ \pm 0.12$) & $1.06$ ($ \pm 0.1$) \\
         & Two-Headed Model + Adaptive Sleep & $-1.93$ ($ \pm 5.46$) & $1.46$ ($ \pm 0.54$) & $1.08$ ($ \pm 0.28$) & $1.05$ ($ \pm 0.19$)  \\
         \hline
        Condensed & Two-Headed Mode & $-5.68$ ($ \pm 2.13$) & $1.42$ ($ \pm 0.1$) & $1.14$ ($ \pm 0.12$) & $1.18$ ($ \pm 0.08$) \\
         & Two-Headed Model + Adaptive Sleep & $-0.53$ ($ \pm 4.49$) & $1.43$ ($ \pm 0.66$) & $1.02$ ($ \pm 0.33$) & $0.87$ ($ \pm 0.17$) \\
         \hline
    \end{tabular}
    }
    \caption{Comparison of the two-headed model with and without self-triggering sleep. Results are averaged over multiple lifetimes and we also record the 95\% confidence interval according to the t-distribution. Each sleep agent used two Eigentasks.}
    \label{tab:self_triggering_sleep_comparison}
\end{table}

\subsubsection{Experience Compression: REMIND}
\begin{table}[H]
    \centering
    \resizebox{\textwidth}{!}{
    \begin{tabular}{|c|c|c|c|c|c|}
        \hline
         Scenario & Agent & PM & FT & BT & RP \\
         \hline
          Pairwise & Two-Headed Model & $-3.35$ ($ \pm 4.3$) & $1.45$ ($ \pm 0.4$) & $0.92$ ($ \pm 0.15$) & $1.12$ ($ \pm 0.21$) \\
         & Two-Headed Model + REMIND & $-2.23$ ($ \pm 2.33$) & $1.58$ ($ \pm 0.22$) & $0.93$ ($ \pm 0.22$) & $0.97$ ($ \pm 0.13$) \\
         \hline
          Alternating & Two-Headed Model & $-8.44$ ($ \pm 5.35$) & $1.04$ ($ \pm 0.31$) & $0.81$ ($ \pm 0.13$) & $0.89$ ($ \pm 0.07$) \\
         & Two-Headed Model + REMIND & $-6.51$ ($ \pm 4.58$) & $1.29$ ($ \pm 0.35$) & $0.78$ ($ \pm 0.2$) & $0.92$ ($ \pm 0.04$) \\
         \hline
        Condensed & Two-Headed Model & $-4.08$ ($ \pm 4.17$) & $1.52$ ($ \pm 0.25$) & $1.2$ ($ \pm 0.47$) & $1.1$ ($ \pm 0.2$) \\
         & Two-Headed Model + REMIND & $-3.67$ ($ \pm 3.92$) & $1.5$ ($ \pm 0.18$) & $1.13$ ($ \pm 0.42$) & $1.11$ ($ \pm 0.18$) \\
         \hline
    \end{tabular}
    }
    \caption{Comparison of the two-headed model with and without a compressed wake experience buffer (REMIND). Results are averaged over 12 lifetimes and we also record the 95\% confidence interval according to the t-distribution. Both agents use pre-training on two tasks not in the test syllabus. Each sleep agent used two Eigentasks.}
    \label{tab:remind_comparison}
\end{table}

\subsubsection{Prioritized Replay for Danger Detection}
\begin{table}[H]
    \centering
    \resizebox{\textwidth}{!}{
    \begin{tabular}{|c|c|c|c|c|c|}
        \hline
         Scenario & Agent & PM & FT & BT & RP \\
         \hline
          Pairwise & Wake & $-0.37$ ($ \pm 2.58$) & $1.62$ ($ \pm 0.38$) & $0.99$ ($ \pm 0.12$) & $1.05$ ($ \pm 0.05$) \\
         & Wake + Danger Detection & $0.39$ ($ \pm 2.18$) & $1.73$ ($ \pm 0.43$) & $1.04$ ($ \pm 0.21$) & $0.98$ ($ \pm 0.05$) \\
         \hline
          Alternating & Wake & $-1.32$ ($ \pm 1.35$) & $1.62$ ($ \pm 0.38$) & $0.96$ ($ \pm 0.07$) & $1.02$ ($ \pm 0.02$)\\
         & Wake + Danger Detection & $1.79$ ($ \pm 2.77$) & $1.73$ ($ \pm 0.43$) & $1.16$ ($ \pm 0.26$) & $0.95$ ($ \pm 0.02$) \\
         \hline
        Condensed & Wake* & $-3.72$ ($ \pm 3.95$) & $1.23$ ($ \pm 0.24$) & $1.0$ ($ \pm 0.07$) & $1.17$ ($ \pm 0.12$) \\
         & Wake + Danger Detection & $0.01$ ($ \pm 2.05$) & $1.55$ ($ \pm 0.34$) & $1.29$ ($ \pm 0.4$) & $1.04$ ($ \pm 0.04$)\\
         \hline
    \end{tabular}
    }
    \caption{Comparison of the wake agent with and without danger detection. Results are averaged over 8 lifetimes and we also record the 95\% confidence interval according to the t-distribution. Each syllabus consists of only ``defeat'' tasks from the SC-2 minigames, with the exclusion of the condensed scenario for the wake-only agent, which is run on tasks starting with two defeat tasks, but include collect tasks within the syllabi.}
    \label{tab:danger_detection_comparison}
\end{table}

\subsubsection{Representation Learning: STAM}
\begin{table}[H]
    \centering
    \resizebox{\textwidth}{!}{
    \begin{tabular}{|c|c|c|c|c|c|}
        \hline
         Scenario & Agent & PM & FT & BT & RP \\
         \hline
          Pairwise & Wake &$-6.82$ ($ \pm 10.43$) & $1.15$ ($ \pm 0.37$) & $0.95$ ($ \pm 0.37$) & $1.01$ ($ \pm 0.09$) \\
         & Wake + STAM & $-4.53$ ($ \pm 6.65$) & $1.48$ ($ \pm 0.33$) & $0.87$ ($ \pm 0.31$) & $0.96$ ($ \pm 0.07$) \\
         \hline
          Alternating & Wake & $-8.34$ ($ \pm 5.37$) & $1.15$ ($ \pm 0.37$) & $0.86$ ($ \pm 0.22$) & $0.91$ ($ \pm 0.09$) \\
         & Wake + STAM & $-1.28$ ($ \pm 2.16$) & $1.48$ ($ \pm 0.33$) & $0.84$ ($ \pm 0.2$) & $0.92$ ($ \pm 0.04$) \\
         \hline
        Condensed & Wake & $-0.09$ ($ \pm 0.33$) & $1.02$ ($ \pm 0.02$) & $1.0$ ($ \pm 0.02$) & $1.07$ ($ \pm 0.07$) \\
         & Wake + STAM & $1.12$ ($ \pm 1.89$) & $1.18$ ($ \pm 0.05$) & $1.1$ ($ \pm 0.09$) & $0.91$ ($ \pm 0.09$) \\
         \hline
    \end{tabular}
    }
    \caption{Comparison of the wake agent with and without STAM. Results are averaged over 12 lifetimes and we also record the 95\% confidence interval according to the t-distribution.}
    \label{tab:stam_comparison}
\end{table}

\subsubsection{Representation Learning: Self-Supervised Learning}

\begin{table}[H]
    \centering
    \resizebox{\textwidth}{!}{
    \begin{tabular}{|c|c|c|c|c|c|}
        \hline
         Scenario & Agent & PM & FT & BT & RP \\
         \hline
          Pairwise & Wake & $-7.47$ ($ \pm 11.45$) & $1.16$ ($ \pm 0.42$) & $0.94$ ($ \pm 0.42$) & $1.01$ ($ \pm 0.11$) \\
         & Wake + SSRL & $-12.75$ ($ \pm 12.46$) & $1.5$ ($ \pm 0.22$) & $0.67$ ($ \pm 0.27$) & $1.09$ ($ \pm 0.11$) \\
         \hline
        Condensed & Wake & $-0.13$ ($ \pm 0.25$) & $1.01$ ($ \pm 0.02$) & $1.0$ ($ \pm 0.02$) & $1.13$ ($ \pm 0.09$) \\
         & Wake + SSRL & $-7.46$ ($ \pm 4.19$) & $1.52$ ($ \pm 0.18$) & $1.37$ ($ \pm 0.42$) & $1.14$ ($ \pm 0.11$) \\
         \hline
         \end{tabular}
    }
    \caption{Comparing the wake agent with and without SSRL. Results are averaged over 12 lifetimes and we also record the 95\% confidence interval according to the t-distribution.}
    \label{tab:ssrl_comparison}
\end{table}

\begin{table}[H]
    \centering
    \resizebox{\textwidth}{!}{
    \begin{tabular}{|c|c|c|c|c|c|}
        \hline
         Scenario & Agent & PM & FT & BT & RP \\
         \hline
          Pairwise & Hidden Replay Model + Pretraining & $-4.63$ ($ \pm 3.76$) & $1.0$ ($ \pm 0.05$) & $0.84$ ($ \pm 0.12$) & $1.07$ ($ \pm 0.12$) \\
         & Wake + SSRL & $-6.52$ ($ \pm 2.67$) & $1.2$ ($ \pm 0.5$) & $0.6$ ($ \pm 0.17$) & $0.91$ ($ \pm 0.07$) \\
         \hline
         \end{tabular}
    }
    \caption{Understanding the performance of SSRL on a small set of pairwise syllabi. Results are averaged over multiple lifetimes and we also record the 95\% confidence interval according to the t-distribution. The comparable baseline model is a hidden replay model with pretraining on the four tasks that do not appear in the pairwise syllabus for each run.}
    \label{tab:ssrl_comparison_2}
\end{table}
